# Supplementary material for: Quasi-symmetry Constrained Spin Ferromagnetism in Altermagnets
Source: arXiv:2412.09338 source file (2025-07-02)
Supplement: Supplementary file 1 [file SM_Quasisym_Constrained_Spin_FM_in_AM.pdf]

# Supplementary Material for: "Quasi-symmetry Constrained Spin Ferromagnetism in Altermagnets"

Mercè Roig,[1] Yue Yu,[2] Rune C. Ekman,[1] Andreas Kreisel,[1] Brian M. Andersen,[1] and Daniel F. Agterberg[2]

[1]*Niels Bohr Institute, University of Copenhagen, DK-2100 Copenhagen, Denmark*

[2]*Department of Physics, University of Wisconsin–Milwaukee, Milwaukee, Wisconsin 53201, USA*

In this supplementary material, we provide details on supporting derivations, resulting analytical expressions for all coefficients in the free energy, extended (quasi)-symmetry analyses, examples of secondary order parameters, general analytic expressions for the Berry curvature and a detailed analysis of the magnetic anisotropy energy.

## S1. GENERAL FREE ENERGY IN THE PRESENCE OF SPIN-ORBIT COUPLING

In the main text we include the form of the free energy for orthorhombic and higher-symmetry groups. In the case of monoclinic groups, there are additional terms due to the lower crystal symmetry, and therefore the free energy can generally be written as

$$f = \frac{a_N}{2}\vec{N}^2 + \frac{b_N}{4}\vec{N}^4 + \frac{a_M}{2}\vec{M}^2 - \vec{h}\cdot\vec{M} + c_{ij}M_iN_j + s_1(N_x^2 - N_y^2) + s_2(N_x^2 + N_y^2 - 2N_z^2) + s_3N_xN_y + s_4N_xN_z + s_5N_yN_z, \tag{S1}$$

where the coefficients $s_3$, $s_4$ and $s_5$ can also be calculated from the general microscopic model and are given by

$$s_3 = -2\sum_{\mathbf{k}} \frac{\lambda_{x,\mathbf{k}}\lambda_{y,\mathbf{k}}}{\tilde{E}_{\mathbf{k}}^2} L(\mathbf{k}), \tag{S2}$$

$$s_4 = -2\sum_{\mathbf{k}} \frac{\lambda_{x,\mathbf{k}}\lambda_{z,\mathbf{k}}}{\tilde{E}_{\mathbf{k}}^2} L(\mathbf{k}), \tag{S3}$$

$$s_5 = -2\sum_{\mathbf{k}} \frac{\lambda_{y,\mathbf{k}}\lambda_{z,\mathbf{k}}}{\tilde{E}_{\mathbf{k}}^2} L(\mathbf{k}). \tag{S4}$$

with the function $L(\mathbf{k}) = \frac{df(\varepsilon)}{d\varepsilon}|_{\varepsilon=E_{\mathbf{k}}^+} + \frac{df(\varepsilon)}{d\varepsilon}|_{\varepsilon=E_{\mathbf{k}}^-} - \frac{2[f(E_{\mathbf{k}}^-)-f(E_{\mathbf{k}}^+)]}{E_{\mathbf{k}}^- - E_{\mathbf{k}}^+}$. Here, $\tilde{E}_{\mathbf{k}} = \sqrt{t_{x,\mathbf{k}}^2 + t_{z,\mathbf{k}}^2 + \vec{\lambda}_{\mathbf{k}}^2}$ are the eigenvalues of $H_1$ and the eigenvalues $E_{\mathbf{k}}^{\pm} = \varepsilon_{0,\mathbf{k}} \pm \tilde{E}_{\mathbf{k}}$ correspond the full Hamiltonian in Eq. (2) of the main text. Note that the coefficients $s_3$, $s_4$ and $s_5$ vanish for higher-symmetry groups.

## S2. FREE ENERGY INVARIANTS COUPLING MAGNETIZATION AND NÉEL ORDER

As discussed in the main text, a bilinear coupling between the magnetization and the Néel order exits if the direct product $\Gamma_A \otimes \Gamma_A \otimes \Gamma_N$ contains the IR transforming trivially under all point group operations, where $\Gamma_A$ is the axial vector irreducible representation (IR) and $\Gamma_N$ is the IR denoting the symmetry of the spin splitting. Equivalently, there is a free energy invariant if $\Gamma_A \otimes \Gamma_A$ contains $\Gamma_N$. In Table S1 we detail the axial vector IR for the different point groups.

As an example, we consider the point group $D_{4h}$. In this case, $\Gamma_A = E_g \oplus A_{2g}$, and therefore $\Gamma_A \otimes \Gamma_A = 3A_{1g} \oplus 2E_g \oplus (E_g \otimes E_g)$. Neither $A_{1g}$ or $E_g$ belong to $\Gamma_N$ (see Table I in the main text), so the invariants can only arise from $E_g \otimes E_g = A_{1g} \oplus A_{2g} \oplus B_{1g} \oplus B_{2g}$. Hence, for each of $\Gamma_N = A_{2g}, B_{1g}, B_{2g}$ there is an allowed bilinear coupling. To illustrate how to obtain the form of the invariant, we focus on the case $\Gamma_N = B_{2g}$. The magnetization $\vec{M}$ belongs to the axial vector IR, and therefore transforms like the spin Pauli matrices, $(M_x, M_y, M_z) \sim (\sigma_x, \sigma_y, \sigma_z)$,

Table S1. Axial vector irreducible representation $\Gamma_A$ and antisymmetric direct product $[\Gamma_A \otimes \Gamma_A]_-$ for all point groups considered in Table I of the main text.

| $P$ | $C_{2h}$ | $D_{2h}$ | $C_{4h}$ | $D_{4h}$ | $D_{3d}$ | $C_{6h}$ | $D_{6h}$ | $O_h$ |
|---|---|---|---|---|---|---|---|---|
| $\Gamma_A$ | $B_g \oplus A_g$ | $B_{1g} \oplus B_{2g} \oplus B_{3g}$ | $A_g \oplus E_g$ | $E_g \oplus A_{2g}$ | $A_{2g} \oplus E_g$ | $A_g \oplus E_{1g}$ | $A_{2g} \oplus E_{1g}$ | $T_{1g}$ |
| $[\Gamma_A \otimes \Gamma_A]_-$ | $B_g$ | $B_{1g} \oplus B_{2g} \oplus B_{3g}$ | $A_g$ | $A_{2g}$ | $A_{2g}$ | $A_g$ | $A_{2g}$ | $T_{1g}$ |

while for the Néel order $(N_x, N_y, N_z) \sim \tau_z(\sigma_x, \sigma_y, \sigma_z)$ (see Eq. (3) in the main text). Since $\tau_z$ transforms like the crystal asymmetric hopping $t_{z,\mathbf{k}}$ it belongs to the IR $\Gamma_N$. Thus, in our particular example $\Gamma_N = B_{2g} \sim k_x k_y$ and $(\sigma_x, \sigma_y, \sigma_z) \sim (k_y k_z, k_x k_z, k_x k_y (k_x^2 - k_y^2))$. As a consequence, the only allowed invariant corresponds to $M_x N_y + M_y N_x$. Following this procedure, we have identified the invariants for the different point groups and symmetries of the altermagnetic spin splitting listed in Table I in the main text.

As seen from Table I in the main text, there are some cases where a bilinear coupling between $\vec{M}$ and $\vec{N}$ is not symmetry allowed. For instance, focusing on the point group $D_{6h}$, the axial IR corresponds to $\Gamma_A = A_{2g} \oplus E_{1g}$. Therefore, $\Gamma_A \otimes \Gamma_A = A_{1g} \oplus 2E_{1g} \oplus (E_{1g} \otimes E_{1g})$, with $E_{1g} \otimes E_{1g} = A_{1g} \oplus A_{2g} \oplus E_{2g}$, which implies that there is only a bilinear coupling for $\Gamma_N = A_{2g}$ and not for $\Gamma_N = B_{1g}, B_{2g}$. Similarly, a bilinear coupling is not allowed for $C_{6h}$ and $O_h$. Consequently, to obtain the lowest-order invariant we have derived the coupling between $\vec{M}$ and $\vec{N}$ to third order. In these cases, an invariant is obtained if $(\Gamma_A \otimes \Gamma_A \otimes \Gamma_A)_{\text{sym}} \otimes \Gamma_A$ contains $\Gamma_N$, where sym denotes the symmetric product of three IRs [1]. The invariant is included in Table I of the main text.

## S3. ANALYTIC EXPRESSION FOR THE COEFFICIENTS IN THE FREE ENERGY FROM MICROSCOPIC MODELS

In this section, we provide the analytic expressions for the coefficients $a_N$, $b_N$ and $a_M$ entering in the free energy in Eq. (1) of the main text using the microscopic model in Eq. (2) and the perturbation in Eq. (3). In the main text, we focus on the interplay between the magnetization and the Néel order, examining the expression for the $c_{ij}$ coefficient, in addition to the coefficients $s_1$ and $s_2$, which determine the magnetic anisotropy energy due to the effect of SOC.

We start by deriving an expression for the free energy density from the partition function $Z$ as

$$\begin{aligned} F &= -\frac{1}{\beta}\log Z = -\frac{1}{\beta}\log\left[\int dc d\bar{c} \exp\left(-cG^{-1}\bar{c}\right)\right] = -\frac{1}{\beta}\log\det\left(G^{-1}\right) = -\frac{1}{\beta}\sum_{i\omega_n}\mathrm{Tr}\log\left(G^{-1}\right) \\ &= -\frac{1}{\beta}\sum_{i\omega_n}\mathrm{Tr}\log\left(G_0^{-1} + H'\right) = -\frac{1}{\beta}\sum_{i\omega_n}\mathrm{Tr}\left[\log\left(G_0^{-1}\right) + \log(1 + G_0 H')\right] \\ &= -\frac{1}{\beta}\sum_{i\omega_n}\mathrm{Tr}\log G_0^{-1} + \frac{1}{2\beta}\sum_{i\omega_n}\mathrm{Tr}\left((G_0 H')^2\right) + \frac{1}{4\beta}\sum_{i\omega_n}\mathrm{Tr}\left((G_0 H')^4\right), \end{aligned}$$

where $G$ is the full Green's function, $G_0$ is the bare Green's function and $H'$ is the perturbation to the normal-state Hamiltonian written in Eq. (3) of the main text, including the Néel order $\vec{N}$ and the induced magnetization $\vec{M}$. In addition, $\beta = 1/k_B T$ and $\omega_n$ corresponds to the Matsubara frequency.

Hence, the second and fourth order corrections to the normal state free energy when the magnetic order sets in are evaluated from

$$F^{(2)} = \frac{1}{2\beta}\sum_{i\omega_n}\mathrm{Tr}[G_0(\mathbf{k}, i\omega_n)H' G_0(\mathbf{k}, i\omega_n)H'], \tag{S5}$$

$$F^{(4)} = \frac{1}{4\beta}\sum_{i\omega_n}\mathrm{Tr}\left[(G_0(\mathbf{k}, i\omega_n)H')^4\right]. \tag{S6}$$

The corresponding diagrammatic representation is illustrated in Fig. S1(a) and (b), respectively, where $\vec{\alpha}$ can denote both order parameters $\vec{N}$ and $\vec{M}$. The bare Green's function projected to the band basis corresponds to

$$G_0(\mathbf{k}, i\omega_n) = \sum_{a=\pm} G_0^a(\mathbf{k}, i\omega_n) \left|u_{\mathbf{k}}^a\right\rangle \left\langle u_{\mathbf{k}}^a\right|, \tag{S7}$$

where $G_0^{(\pm)}(\mathbf{k}, i\omega_n) = \frac{1}{i\omega_n - (\varepsilon_{0,\mathbf{k}} \pm \tilde{E}_{\mathbf{k}})}$ denotes the Green's function in the band basis, with the two-fold degenerate eigenenergies $E_{\mathbf{k}}^{\pm} = \varepsilon_{0,\mathbf{k}} \pm \tilde{E}_{\mathbf{k}}$ where $\tilde{E}_{\mathbf{k}} = \sqrt{t_{x,\mathbf{k}}^2 + t_{z,\mathbf{k}}^2 + \vec{\lambda}_{\mathbf{k}}^2}$ are the eigenenergies of $H_1 = t_{x,\mathbf{k}}\tau_x + t_{z,\mathbf{k}}\tau_z + \tau_y \vec{\lambda}_{\mathbf{k}} \cdot \vec{\sigma}$. With this, we construct the projection operator [2, 3]

$$P_{\mathbf{k}}^a = \left|u_{\mathbf{k}}^a\right\rangle \left\langle u_{\mathbf{k}}^a\right| = \frac{1}{4}\left(\mathbb{1} + \frac{H_1}{\pm\tilde{E}_{\mathbf{k}}}\right) \tag{S8}$$

from sublattice basis onto band $a$ at wavevector $\mathbf{k}$.

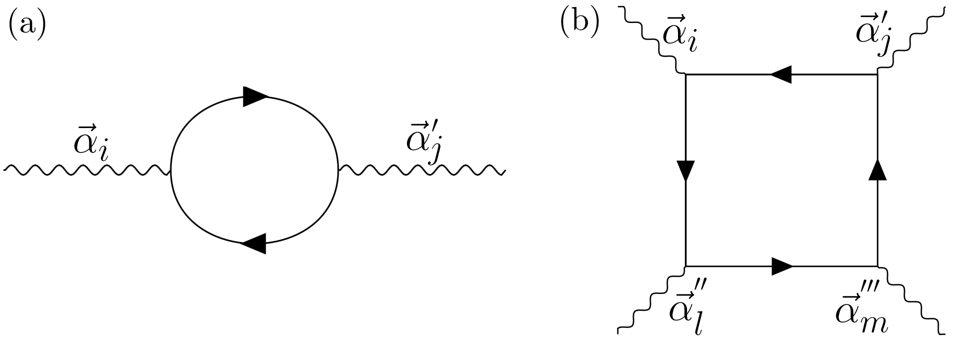


Figure S1. (a) Second-order and (b) fourth-order diagrams contributing to the free energy expansion where $\vec{\alpha}_i$, $\vec{\alpha}'_j$, $\vec{\alpha}''_l$ and $\vec{\alpha}'''_m$ can denote the components of the two magnetic orders $\vec{M}$ and $\vec{N}$.

We focus first on the term coupling the two Néel order parameters $\vec{N}$ corresponding to the coefficient $a_N$ in the free energy, obtaining

$$F_N^{(2)} = \frac{\vec{N}^2}{\beta} \sum_{i\omega_n} \mathrm{Tr}\left[ \sum_{a,b} G^a(\mathbf{k}, i\omega_n) G^b(\mathbf{k}, i\omega_n) \tau_z \left|u^a_{\mathbf{k}}\right\rangle \left\langle u^a_{\mathbf{k}}\right| \tau_z \left|u^b_{\mathbf{k}}\right\rangle \left\langle u^b_{\mathbf{k}}\right| \right], \tag{S9}$$

where we have replaced the Green's function projected in the band basis (see Eq. (S7)) into Eq. (S5). Note that the trace is over all degrees of freedom, including $\mathbf{k}$ and the Matsubara frequency $i\omega_n$. Using the projector operator written in Eq. (S8), the expression for the free energy can be simplified to

$$F_N^{(2)} = \frac{\vec{N}^2}{\beta} \sum_{\mathbf{k}, i\omega_n} \frac{1}{t^2_{x,\mathbf{k}} + t^2_{z,\mathbf{k}}} \Big( 2t^2_{x,\mathbf{k}} G^-(\mathbf{k}, i\omega_n) G^+(\mathbf{k}, i\omega_n) + t^2_{z,\mathbf{k}} \big[ (G^-(\mathbf{k}, i\omega_n))^2 + (G^+(\mathbf{k}, i\omega_n))^2 \big] \Big). \tag{S10}$$

Hence, performing the Matsubara frequency sum we identify

$$a_N = \frac{1}{U} + 2\sum_{\mathbf{k}} \frac{1}{t^2_{x,\mathbf{k}} + t^2_{z,\mathbf{k}}} \left\{ t^2_{x,\mathbf{k}} \frac{2\big[f\big(E^-_{\mathbf{k}}\big) - f\big(E^+_{\mathbf{k}}\big)\big]}{E^-_{\mathbf{k}} - E^+_{\mathbf{k}}} + t^2_{z,\mathbf{k}} \left[ \left.\frac{df(\varepsilon)}{d\varepsilon}\right|_{\varepsilon = E^+_{\mathbf{k}}} + \left.\frac{df(\varepsilon)}{d\varepsilon}\right|_{\varepsilon = E^-_{\mathbf{k}}} \right] \right\}, \tag{S11}$$

with $f\big(E^a_{\mathbf{k}}\big)$ denoting the Fermi function evaluated for the energy band $a$. Here, $\frac{1}{U}$ is the bare bosonic contribution from the Hubbard–Stratonovich transformation. This expression reveals that the susceptibility depends on the competition between the inter-band term and the intra-band term, as discussed in Ref. [3], and this determines whether ferromagnetism or Néel order is stabilized. Additionally, it also shows that band degeneracies help stabilizing altermagnetism.

We can follow the same procedure to obtain the $a_M$ coefficient by focusing on the magnetization term in the perturbation. Thus, the free energy now simply reads

$$F_M^{(2)} = \frac{\vec{M}^2}{\beta} \sum_{\mathbf{k}, i\omega_n} [(G^-(\mathbf{k}, i\omega_n))^2 + (G^+(\mathbf{k}, i\omega_n))^2]. \tag{S12}$$

Similarly to the previous case, the expression for the coefficient corresponds to

$$a_M = \frac{1}{U} + 2\sum_{\mathbf{k}} \left\{ \left.\frac{df(\varepsilon)}{d\varepsilon}\right|_{\varepsilon = E^+_{\mathbf{k}}} + \left.\frac{df(\varepsilon)}{d\varepsilon}\right|_{\varepsilon = E^-_{\mathbf{k}}} \right\}. \tag{S13}$$

In contrast to Eq. (S11), this coefficient contains only an intra-band term.

Finally, we can use Eq. (S6) to derive an expression for the quartic contribution to the free energy from the microscopic model, which corresponds to the diagram in Fig. S1(b). In this case, the expression for the coefficient $b_N$

in the free energy expansion corresponds to

$$b_N = 4\sum_{\mathbf{k}} \frac{1}{(t_{x,\mathbf{k}}^2 + t_{z,\mathbf{k}}^2)^2} \Bigg\{ \frac{t_{x,\mathbf{k}}^4}{(E_{\mathbf{k}}^- - E_{\mathbf{k}}^+)^2} \left( f'(\varepsilon)\Big|_{\varepsilon=E_{\mathbf{k}}^+} + f'(\varepsilon)\Big|_{\varepsilon=E_{\mathbf{k}}^-} - 2\frac{f(E_{\mathbf{k}}^-) - f(E_{\mathbf{k}}^+)}{E_{\mathbf{k}}^- - E_{\mathbf{k}}^+} \right) + \frac{t_{z,\mathbf{k}}^4}{12} \left( f'''(\varepsilon)\Big|_{\varepsilon=E_{\mathbf{k}}^+} + f'''(\varepsilon)\Big|_{\varepsilon=E_{\mathbf{k}}^-} \right)$$
$$+ \frac{t_{x,\mathbf{k}}^2 t_{z,\mathbf{k}}^2}{E_{\mathbf{k}}^- - E_{\mathbf{k}}^+} \left( f''(\varepsilon)\Big|_{\varepsilon=E_{\mathbf{k}}^+} + f''(\varepsilon)\Big|_{\varepsilon=E_{\mathbf{k}}^-} - \frac{4}{E_{\mathbf{k}}^- - E_{\mathbf{k}}^+} \left[ f'(\varepsilon)\Big|_{\varepsilon=E_{\mathbf{k}}^+} + f'(\varepsilon)\Big|_{\varepsilon=E_{\mathbf{k}}^-} \right] + 8\frac{f(E_{\mathbf{k}}^-) - f(E_{\mathbf{k}}^+)}{(E_{\mathbf{k}}^- - E_{\mathbf{k}}^+)^2} \right) \Bigg\}. \tag{S14}$$

## S4. SOC-ENABLED QUASI-SYMMETRY

In this section, we provide general quasi-symmetry criteria beyond what is used in the main text. The quasi-symmetry criteria comes from the following properties in the normal-state Hamiltonian. In the normal-state band projector and Green's function (Eq. (S8)), the SOC-linear contribution appears as a linear combination of the three SOC terms. Cross-terms like $\sqrt{\lambda_x \lambda_y}$ are absent here. Consequently, any quantities derived from the normal-state Green's function should exhibit the same behavior. In other words, the SOC-linear contributions to any Landau parameters and any linear response coefficients are always expressed as a linear combination of $\lambda_{x,y,z}$. This property is consistent across all the minimal models used in this study.

### A. Quasi-symmetry used in the main text

The $\lambda_x$ linear contribution, specifically, should then exist by itself, even when the other two SOC terms are taken to be exactly zero. When setting the other two SOC terms to zero, the resulting normal-state Hamiltonian gains additional symmetries: spin-rotational symmetries of arbitrary angles along the $x$-axis. If a Landau term is odd under any of these additional quasi-symmetries, then the corresponding Landau coefficient cannot host pure $\lambda_x$ contribution, including $\lambda_x^1$, $\lambda_x^2$, $\lambda_x^3$ and so on. Similarly, spin rotational symmetry along the $y$- (or $z$)-axis can be used to rule out pure $\lambda_y$ (or $\lambda_z$) contributions. If a Landau coefficient has no pure $\lambda_{x,y,z}$ contributions, then it must be at least quadratic in SOC.

### B. General quasi-symmetry

The quasi-symmetry criteria described above provide a sufficient, but not necessary, condition to eliminate SOC-linear contributions. These criteria exclude not only SOC-linear terms such as $\lambda_{x,y,z}$ but also any contributions involving pure $\lambda_i$ terms, like $\lambda_x^3$. However, if a Landau coefficient's leading contribution is $\lambda_x^3$, the quasi-symmetry argument above cannot confirm the absence of SOC-linear contributions. To address this, we develop a more general quasi-symmetry criterion specifically aimed at identifying SOC-linear contributions.

As an example, consider the Landau term $M_xN_x - M_yN_y$, which is relevant for the site symmetry $B_{1g}$ in $D_{4h}$. We aim to demonstrate the absence of SOC-linear contributions to this coefficient. Based on the properties of the normal-state band projector, checking for $\lambda_x$-linear contributions reduces to analyzing the coefficient of $(M_xN_x - M_yN_y)M_xO_x$ in the absence of any SOC. The presence of a $\lambda_x$-linear contribution would manifest through the inclusion of an additional $M_xO_x$ factor. Importantly, no further SOC terms are included in this analysis. For completeness, we also account for a factor $O_x$ from the real-space component of the SOC $\lambda_x$, though this will not influence the subsequent discussion.

The absence of SOC leads to arbitrary spin-rotational symmetry. The term $(M_xN_x - M_yN_y)M_x$ is odd under spin rotation $C_{2y}^{\text{spin}}$, so it must vanish. This implies the absence of $\lambda_x$-linear contribution to $(M_xN_x - M_yN_y)$. Similarly, to check the $\lambda_y$-linear contribution, we need to analyze $(M_xN_x - M_yN_y)M_y$ in the absence of any SOC. The term $(M_xN_x - M_yN_y)M_y$ is odd under spin rotation $C_{2x}^{\text{spin}}$, implying the absence of $\lambda_y$-linear contribution to $(M_xN_x - M_yN_y)$. For the $\lambda_z$-linear contribution, we need to analyze $(M_xN_x - M_yN_y)M_z$. This term is odd under $C_{2x}^{\text{spin}}$, preventing the $\lambda_z$-linear contribution to $(M_xN_x - M_yN_y)$. Therefore, $M_xN_x - M_yN_y$ has no SOC-linear contributions.

For completeness, let us also consider the term $M_zN_y^3$, which is relevant for the site symmetry $B_{1g}$ in $D_{6h}$. The absence of $\lambda_y$ and $\lambda_z$ contributions follows from the same quasi-symmetry argument in the main text, where $C_{2y}^{\text{spin}}$ (or $C_{2z}^{\text{spin}}$) rules out pure-$\lambda_y$ (or $\lambda_z$) contributions. However, for $\lambda_x$, the quasi-symmetry argument in the main text

is insufficient because $M_z N_y^3$ is not odd under any spin rotation along $x$. Instead, the more general quasi-symmetry argument applies. Specifically, we analyze the Landau term $M_z N_y^3 M_x$. This term is odd under $C_{4y}^{\text{spin}}$, ruling out the $\lambda_x$-linear contribution to the coefficient of $M_z N_y^3$. Numerical study reveals a $\lambda_x^3$ contribution to this coefficient.

These examples demonstrate that SOC-linear contributions are possible only if the corresponding term forms a component of a spin vector. For instance, $M_x N_y - M_y N_x$ is the $z$-component of $\mathbf{M} \times \mathbf{N}$. Since $(\mathbf{M} \times \mathbf{N}) \cdot \mathbf{M}$ is allowed under arbitrary spin-rotational symmetry, $M_x N_y - M_y N_x$ can have a $\lambda_z$-linear coefficient. This analysis can be extended to other types of SOC dependence. For example, to check for a $\lambda_x \times \lambda_y$ contribution to the coefficient of a Landau term $O$, one can analyze the coefficient of $O M_x M_y$ under arbitrary spin rotations.

## S5. SECONDARY ORDER PARAMETERS

When a primary order parameter sets in, secondary order parameters are also induced by symmetry. As seen from Eq. (9) of the main text, these secondary order parameters can induce a finite coupling between the Néel order $\vec{N}$ and the magnetization $\vec{M}$. In this section, we focus on the tetragonal example with point group $P = D_{4h}$ and a symmetry for the spin splitting belonging to $\Gamma_N = B_{2g} \sim k_x k_y$, which is relevant for the rutile lattice (SG 136), and detail the form of the allowed secondary order parameters.

Since in this case $M_y$ and $N_x$ transform like $\sigma_y$, $N_x \sim \tau_z \sigma_x$ can induce $M_y$ through 10 different secondary order parameters breaking time-reversal symmetry: $\sin k_x \sin k_y \tau_0 \sigma_x$, $\sin k_x \sin k_y \tau_z \sigma_y$, $\sin k_y \sin k_z \tau_0 \sigma_z$, $\cos\frac{k_x}{2} \sin\frac{k_y}{2} \sin\frac{k_z}{2} \tau_x \sigma_z$, $\sin k_x \sin k_z \tau_z \sigma_z$, $\sin k_y \sin k_z (\cos k_x - \cos k_y) \tau_0 \sigma_z$, $\sin k_x \sin k_z (\cos k_x - \cos k_y) \tau_z \sigma_z$, $(\cos k_x - \cos k_y) \tau_z \sigma_x$, $(\cos k_x - \cos k_y) \tau_0 \sigma_y$, and $\cos\frac{k_x}{2} \sin\frac{k_y}{2} \sin\frac{k_z}{2} \tau_y$. Remarkably, the last one corresponds to a pure orbital current state that couples to the Néel order, but there are other orders with different spin textures. Notably, $(\cos k_x - \cos k_y) \tau_z \sigma_x$ is able to couple to $\tau_z \sigma_x$ with a coefficient quadratic in SOC and it also couples to $\tau_0 \sigma_y$ with a coefficient linear in SOC.

Among them, quadratic SOC dependence of the FM spin moment can be obtained through 4 secondary order parameters: $\sin k_x \sin k_y \tau_0 \sigma_x$, $\sin k_x \sin k_y \tau_z \sigma_y$, $\cos\frac{k_x}{2} \sin\frac{k_y}{2} \sin\frac{k_z}{2} \tau_x \sigma_z$, and $\cos\frac{k_x}{2} \sin\frac{k_y}{2} \sin\frac{k_z}{2} \tau_y$. Other secondary order parameters lead to cubic SOC dependence of the FM spin moment.

## S6. HOPPING PARAMETERS AND SOC FOR THE RUTILE LATTICE AND $FeSb_2$

The general form for the normal-state Hamiltonian describing altermagnetism is given in Eq. (2) of the main text. In Tables S2 - S3 we detail the relevant form for the hoppings and spin-orbit coupling for the rutile lattice (SG 136) and $FeSb_2$ (SG 58) used to obtain the band structures and the magnetizations as a function of the SOC strength shown in Fig. (2) of the main text.

In order to estimate the SOC for $FeSb_2$, we perform DFT calculations using Wien2k [4] (SG 58, $a = 5.8379$Å $b = 6.5248$Å, $c = 3.1811$Å, internal position $(x, y, z) = (0.20094827, 0.35723599, 0)$ for Sb on Wyckoff position 4g), and read off the splittings induced by the spin-orbit terms at $\mathbf{k}_1 = (\pi, 0, \pi)$ where $t_{x,\mathbf{k}_1} = t_{z,\mathbf{k}_1} = \lambda_{y,\mathbf{k}_1} = \lambda_{z,\mathbf{k}_1} = 0$ and the splitting is solely induced by $\lambda_{x,\mathbf{k}_1} = \lambda_x$. Similarly, at $\mathbf{k}_2 = (0, \pi, \pi)$, we have $t_{x,\mathbf{k}_2} = t_{z,\mathbf{k}_2} = \lambda_{x,\mathbf{k}_2} = \lambda_{z,\mathbf{k}_2} = 0$ and the splitting is given by $\lambda_{y,\mathbf{k}_2} = \lambda_y$. Finally, for $\lambda_z$ we use the self-consistently converged densities in the DFT calculation with SOC, but calculate the eigenenergies without including the SOC perturbatively. The energy shift $\Delta E$ of the band positions with and without SOC at the $\Gamma$ point is given by $\Delta E = \sqrt{t_8^2 + \lambda_z^2} - |t_8|$ since the other components of the SOC vanish. Using that $t_8 = 0.15$ eV, we obtain $\vec{\lambda}_0 = (2.7, 6.6, 75)$ meV as used for the calculations in the main text.

Table S2. Tight-binding hoppings and SOC entering in the minimal model in Eq. (2) of the main text relevant for the rutile lattice and $FeSb_2$, as identified in Ref. [3]. The hopping and SOC parameters are detailed in Table S3.

| | **Rutile lattice** | **$FeSb_2$** |
|---|---|---|
| $t_{x,\mathbf{k}}$ | $t_8 \cos\frac{k_x}{2} \cos\frac{k_y}{2} \cos\frac{k_z}{2}$ | |
| $t_{z,\mathbf{k}}$ | $t_6 \sin k_x \sin k_y + t_7 \sin k_x \sin k_y \cos k_z$ | |
| $\lambda_{x,\mathbf{k}}$ | $\lambda \sin\frac{k_z}{2} \sin\frac{k_x}{2} \cos\frac{k_y}{2}$ | $\lambda_x \sin\frac{k_z}{2} \sin\frac{k_x}{2} \cos\frac{k_y}{2}$ |
| $\lambda_{y,\mathbf{k}}$ | $-\lambda \sin\frac{k_z}{2} \sin\frac{k_y}{2} \cos\frac{k_x}{2}$ | $\lambda_y \sin\frac{k_z}{2} \sin\frac{k_y}{2} \cos\frac{k_x}{2}$ |
| $\lambda_{z,\mathbf{k}}$ | $\lambda_z \cos\frac{k_z}{2} \cos\frac{k_x}{2} \cos\frac{k_y}{2} (\cos k_x - \cos k_y)$ | $\lambda_z \cos\frac{k_z}{2} \cos\frac{k_x}{2} \cos\frac{k_y}{2}$ |
| $\varepsilon_{0,\mathbf{k}}$ | $t_1(\cos k_x + \cos k_y) + t_2 \cos k_z + t_3 \cos k_x \cos k_y$ $+ t_4(\cos k_x + \cos k_y) \cos k_z$ $+ t_5 \cos k_x \cos k_y \cos k_z - \mu$ | $t_{1,x} \cos k_x + t_{1,y} \cos k_y + t_2 \cos k_z$ $+ t_3 \cos k_x \cos k_y + t_{4,x} \cos k_x \cos k_z$ $+ t_{4,y} \cos k_y \cos k_z + t_5 \cos k_x \cos k_y \cos k_z - \mu$ |

Table S3. Tight-binding hopping parameters in units of eV found in Ref. [3] used to obtain the band structures in Fig. (1) of the main text and Figs. S4-S5. The SOC parameters estimated from DFT results.

| $RuO_2$ | $t_1$ | | $t_2$ | $t_3$ | $t_4$ | | $t_5$ | $t_6$ | $t_7$ | $t_8$ | $\mu$ | $\lambda$ | | $\lambda_z$ |
|---|---|---|---|---|---|---|---|---|---|---|---|---|---|---|
| | -0.05 | | 0.7 | 0.5 | -0.15 | | -0.4 | -0.6 | 0.3 | 1.7 | 0.25 | 0.05 | | 0.17 |
| $FeSb_2$ | $t_{1,x}$ | $t_{1,y}$ | $t_2$ | $t_3$ | $t_{4,x}$ | $t_{4,y}$ | $t_5$ | $t_6$ | $t_7$ | $t_8$ | $\mu$ | $\lambda_x$ | $\lambda_y$ | $\lambda_z$ |
| | -0.1 | -0.05 | -0.05 | 0.06 | 0.1 | 0.05 | -0.05 | 0.05 | -0.1 | 0.15 | -0.12 | 0.0027 | 0.0066 | 0.075 |

For $RuO_2$, we use the same procedure, i.e. a DFT calculation using Wien2k [4] (SG 136, $a = 4.4825$Å, $c = 3.1113$Å, internal position $(x, y, z) = (0.30544216, 0.30544216, 0)$ for O on Wyckoff position 4f, and Ru on Wyckoff postion 2a), once with spin-orbit coupling and once without it. We then find $\lambda$ at the point $\mathbf{k}_3 = (\pi, 0, \pi)$ where all but $\lambda_{x,\mathbf{k}}$ vanish. $\lambda_z$ is here identified at the point $\mathbf{k}_4 = (\frac{\pi}{2}, 0, 0)$ where $\Delta E = \frac{1}{\sqrt{2}}(\sqrt{t_8^2 + \lambda_z^2} - |t_8|)$. For $RuO_2$ we then obtain $\vec{\lambda}_0 = (0.05, 0.05, 0.17)$ eV.

## S7. GENERAL EXPRESSIONS FOR THE BERRY CURVATURE

In the presence of SOC, the Néel order $\vec{N}$ induces a FM order $\vec{M}$. Focusing on the previous cases of the rutile lattice and $FeSb_2$, the free energy invariant corresponds to $M_xN_y + M_yN_x$. Therefore, an in-plane Néel order $\vec{N} = (N_x, 0, 0)$ induces a magnetization $\vec{M} = (0, M_y, 0)$. In the presence of these orders, the Hamiltonian without including the dispersion corresponds to

$$H = t_{x,\mathbf{k}}\tau_x + t_{z,\mathbf{k}}\tau_z + \tau_y\vec{\lambda}_\mathbf{k}\cdot\vec{\sigma} + M_y\sigma_y + N_x\tau_z\sigma_x, \tag{S15}$$

with

$$E_{\alpha=\pm,\beta=\pm} = \alpha\left(N_x^2+M_y^2+\vec{\lambda}_\mathbf{k}^2+t_{x,\mathbf{k}}^2+t_{z,\mathbf{k}}^2+\beta 2\sqrt{N_x^2\left(\lambda_{z,\mathbf{k}}^2+\lambda_{y,\mathbf{k}}^2+t_{z,\mathbf{k}}^2\right)+M_y^2\left(\lambda_{y,\mathbf{k}}^2+t_{z,\mathbf{k}}^2+t_{x,\mathbf{k}}^2\right)-2N_xM_y\lambda_{z,\mathbf{k}}t_{x,\mathbf{k}}}\right)^{1/2}. \tag{S16}$$

The general lowest-order expression for the Berry curvature is given by [2]

$$\begin{aligned}\Omega_{\alpha,\beta,ij} = \sum_{m,n=i,j}\varepsilon_{mn}\Bigg[&\frac{3M_y}{8E_2}\left(\frac{\beta(N_x^2+M_y^2)}{3E_2^2}+\frac{\beta N_x^2(N_x^2+t_{x,\mathbf{k}}^2+2M_y^2)+M_y^4}{E_{\alpha\beta}^2E_2^2}+\frac{2(N_x^2+M_y^2)}{E_{\alpha\beta}^2E_2}+\frac{\beta}{E_{\alpha\beta}^2}\right)\\ &(\lambda_{y,\mathbf{k}}\partial_m t_{x,\mathbf{k}}\partial_n t_{z,\mathbf{k}}+t_{x,\mathbf{k}}\partial_m t_{z,\mathbf{k}}\partial_n\lambda_{y,\mathbf{k}}+t_{z,\mathbf{k}}\partial_m\lambda_{y,\mathbf{k}}\partial_n t_{x,\mathbf{k}})\\ &+\frac{N_xt_{z,\mathbf{k}}}{8E_{\alpha\beta}^3}\left(\frac{\beta(N_x^2t_{z,\mathbf{k}}^2+M_y^2(t_{x,\mathbf{k}}^2+t_{z,\mathbf{k}}^2))}{E_2^3}+\frac{3\beta}{E_2}\right)(\lambda_{x,\mathbf{k}}\partial_m t_{x,\mathbf{k}}\partial_n t_{z,\mathbf{k}}+t_{x,\mathbf{k}}\partial_m t_{z,\mathbf{k}}\partial_n\lambda_{x,\mathbf{k}}+t_{z,\mathbf{k}}\partial_m\lambda_{x,\mathbf{k}}\partial_n t_{x,\mathbf{k}})\\ &+\frac{N_x}{8E_{\alpha\beta}^3}\left(\frac{3N_x^2t_{z,\mathbf{k}}^2+3M_y^2(t_{x,\mathbf{k}}^2+t_{z,\mathbf{k}}^2)}{E_2^2}+1\right)(\partial_m\lambda_{x,\mathbf{k}}\partial_n t_{x,\mathbf{k}})\Bigg],\end{aligned} \tag{S17}$$

where we introduced

$$E_2 = \sqrt{N_x^2\left(\lambda_{z,\mathbf{k}}^2+\lambda_{y,\mathbf{k}}^2+t_{z,\mathbf{k}}^2\right)+M_y^2\left(\lambda_{y,\mathbf{k}}^2+t_{z,\mathbf{k}}^2+t_{x,\mathbf{k}}^2\right)-2N_xM_y\lambda_{z,\mathbf{k}}t_{x,\mathbf{k}}}, \tag{S18}$$

which has units of energy squared. When $M_y = 0$, Eq. (S17) reduces to

$$\begin{aligned}\Omega_{\alpha,\beta,ij} =& \frac{1}{8E_{\alpha,\beta}^3}\sum_{m,n=i,j}\varepsilon_{mn}\Bigg[\left(N_x+\frac{3N_xt_{z,\mathbf{k}}^2}{E_1^2}+\frac{3\beta t_{z,\mathbf{k}}^2}{E_1}+\frac{\beta t_{z,\mathbf{k}}^4}{E_1^3}\right)\partial_m\lambda_{x,\mathbf{k}}\partial_n t_{x,\mathbf{k}}+\left(\frac{3\beta\lambda_xt_{z,\mathbf{k}}}{E_1}+\frac{\beta\lambda_xt_{z,\mathbf{k}}^3}{E_1^3}\right)\partial_m t_{x,\mathbf{k}}\partial_n t_{z,\mathbf{k}}\\ &+\left(\frac{3\beta t_{x,\mathbf{k}}t_{z,\mathbf{k}}}{E_1}+\frac{\beta t_{x,\mathbf{k}}t_{z,\mathbf{k}}^3}{E_1^3}\right)\partial_m t_{z,\mathbf{k}}\partial_n\lambda_{x,\mathbf{k}}\Bigg],\end{aligned} \tag{S19}$$

which includes SOC components in all direction and where now $E_1 = \sqrt{t_{z,\mathbf{k}}^2 + \lambda_{z,\mathbf{k}}^2 + \lambda_{y,\mathbf{k}}^2}$. For $\lambda_{y,\mathbf{k}} = \lambda_{z,\mathbf{k}} = 0$, this expression further reduces to Eq. (10) in the main text.

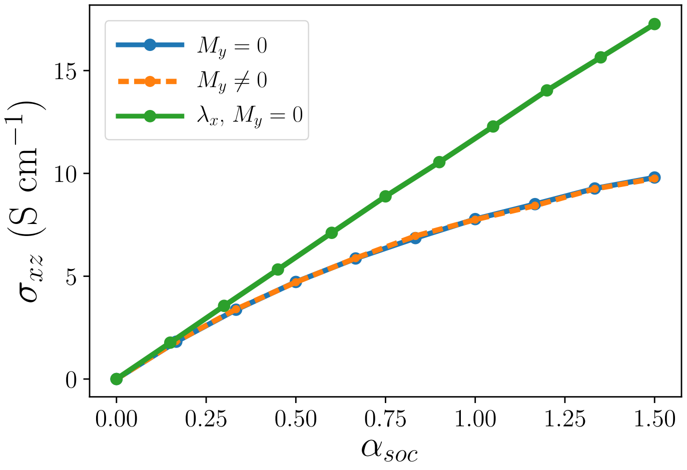


Figure S2. Hall conductivity as a function of SOC strength for $RuO_2$, considering the tight-binding model and parameters in Tables S2-S3. We take $\vec{\lambda} = \alpha_{soc}\vec{\lambda}_0$ with $\vec{\lambda}_0 = (0.05, 0.05, 0.17)$ eV and $N_x = 0.2$ eV. The orange (blue) line corresponds to the Berry curvature in Eq. (S17) (Eq. (S19)). The green line is obtained from the Berry curvature in Eq. (S19) considering only SOC in the $x$-direction.

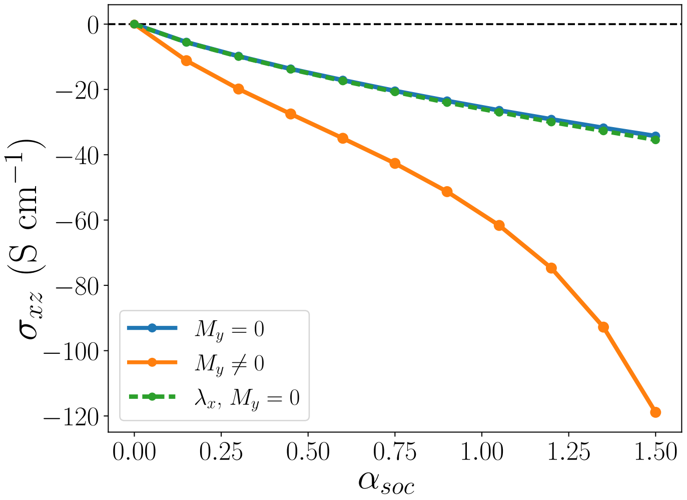


Figure S3. Hall conductivity as a function of SOC strength for $FeSb_2$, considering the tight-binding model and parameters in Tables S2-S3. We take $\vec{\lambda} = \alpha_{soc}\vec{\lambda}_0$ with $\vec{\lambda}_0 = (0.0027, 0.0066, 0.075)$ eV and $N_x = 0.05$ eV. The orange (blue) line corresponds to the Berry curvature in Eq. (S17) (Eq. (S19)). The green line is obtained from the Berry curvature in Eq. (S19) considering only SOC in the $x$-direction.

We have additionally considered the Berry curvature in the presence of only an in-plane $M_y$ magnetization. In this case, Eq. (S17) reduces to

$$\Omega^{(M_y)}_{\alpha,\beta,ij} = \frac{\mathrm{sgn}(M_y)\beta}{8\tilde{E}^3} \sum_{m,n=i,j} \varepsilon_{mn} \left[ \left( 1 + \frac{3}{E^2_{\alpha,\beta}} (\tilde{E}_y + \beta|M_y|)^2 \right) (t_{z,\mathbf{k}} \partial_m \lambda_{y,\mathbf{k}} \partial_n t_{x,\mathbf{k}} + t_{x,\mathbf{k}} \partial_m t_{z,\mathbf{k}} \partial_n \lambda_{y,\mathbf{k}} + \lambda_{y,\mathbf{k}} \partial_m t_{x,\mathbf{k}} \partial_n t_{z,\mathbf{k}}) \right], \tag{S20}$$

and the Berry curvature is also linear in the SOC component parallel to the magnetization. In the previous expression, $\tilde{E}_y = \sqrt{t^2_{z,\mathbf{k}} + t^2_{x,\mathbf{k}} + \lambda^2_{y,\mathbf{k}}}$ and $E_{\alpha=\pm,\beta=\pm}$ is now Eq. (S16) in the case $N_x = 0$. The dispersion of the spin up and spin down bands is different in the presence of $\vec{M}$, and consequently this term also give rise to a finite AHE.

In Figs. S2-S3 we show the Hall conductivity for the rutile lattice and the $FeSb_2$ tight-binding models (see Tables S2-

S3), calculated from the Berry curvature as

$$\sigma_{ij} = -\frac{e^2}{\hbar}\int_{\mathrm{BZ}} \frac{d\mathbf{k}}{(2\pi)^3} \sum_{\alpha,\beta} f_{\alpha,\beta}(\mathbf{k})\Omega_{\alpha,\beta,ij}, \tag{S21}$$

where $f_{\alpha,\beta}(\mathbf{k})$ is the Fermi-Dirac contribution of each band $\alpha, \beta$. In the case of $RuO_2$ ($P = D_{4h}$, $\Gamma_N = B_{2g}$), see Fig. S2, Eqs. (S17) and (S19) yield almost the same result for the conductivity. Therefore, the induced magnetization for this tetragonal material does not give rise to a significant contribution to the anomalous Hall conductivity, as expected from Table I in the main text, since $\vec{M}$ is induced to second (or higher order) in the SOC. In contrast, if we focus on the band structure inspired by $FeSb_2$ ($P = D_{2h}$, $\Gamma_N = B_{1g}$), the induced magnetization $\vec{M}$ is allowed to linear order in SOC (see Table I in the main text) and may give rise to significant contributions to the anomalous Hall conductivity, as seen from Fig. S3.

## S8. MAGNETIC ANISOTROPY ENERGY

In this section, we derive the expression for the magnetic anisotropy energy and examine the preferred direction using microscopic models relevant for the rutile lattice (SG 136) and $FeSb_2$ (SG 58). In the presence of the Néel order parameter and SOC the free energy is given by

$$F = s_x N_x^2 + s_y N_y^2 + s_z N_z^2. \tag{S22}$$

In Eq. (1) of the main text we rewrite this expression in the form

$$F = s_0(N_x^2 + N_y^2 + N_z^2) + s_1(N_x^2 - N_y^2) + s_2(N_x^2 + N_y^2 - 2N_z^2), \tag{S23}$$

so that the coefficients $s_0$, $s_1$ and $s_2$ correspond to

$$\begin{aligned} s_0 &= \frac{1}{3}(s_x + s_y + s_z),\\ s_1 &= \frac{1}{2}(s_x - s_y),\\ s_2 &= \frac{1}{6}(s_x + s_y - 2s_z). \end{aligned} \tag{S24}$$

The expression for the coefficients is derived from the following contribution of the free energy to second order (see Fig. S1(a)),

$$F_J^{(2)} = \frac{1}{2\beta}\sum_{i\omega_n} \mathrm{Tr}\left[\sum_{a,b} G^a(\mathbf{k}, i\omega_n)G^b(\mathbf{k}, i\omega_n)\tau_z\vec{N}\cdot\vec{\sigma}P^a_{\mathbf{k}}\tau_z\vec{N}\cdot\vec{\sigma}P^b_{\mathbf{k}}\right], \tag{S25}$$

where $G^a(\mathbf{k}, i\omega_n)$ and $P^a_{\mathbf{k}}$ are the Green's function and the projector operator defined in Eq. (S7) and Eq. (S8), respectively. In particular, we are concerned with the corrections due to SOC, and therefore we specifically analyze the trace

$$\begin{aligned} &\frac{1}{16}\mathrm{Tr}\Big[\tau_z\vec{N}\cdot\vec{\sigma}\tau_y\vec{\lambda}_{\mathbf{k}}\cdot\vec{\sigma}\tau_z\vec{N}\cdot\vec{\sigma}\tau_y\vec{\lambda}_{\mathbf{k}}\cdot\vec{\sigma}\Big]\\ &= -\frac{1}{4}\Big\{N_x^2(\lambda_{x,\mathbf{k}}^2 - \lambda_{y,\mathbf{k}}^2 - \lambda_{z,\mathbf{k}}^2) + N_y^2(-\lambda_{x,\mathbf{k}}^2 + \lambda_{y,\mathbf{k}}^2 - \lambda_{z,\mathbf{k}}^2) + N_z^2(-\lambda_{x,\mathbf{k}}^2 - \lambda_{y,\mathbf{k}}^2 + \lambda_{z,\mathbf{k}}^2)\\ &\quad + 4(N_xN_y\lambda_{x,\mathbf{k}}\lambda_{y,\mathbf{k}} + N_xN_z\lambda_{x,\mathbf{k}}\lambda_{z,\mathbf{k}} + N_yN_z\lambda_{y,\mathbf{k}}\lambda_{z,\mathbf{k}})\Big\}. \end{aligned} \tag{S26}$$

From this expression, the general form of the free energy in Eq. (S1) directly follows. Focusing on orthorhombic or higher-symmetry groups, the form for the $s_x$, $s_y$ and $s_z$ coefficients in Eq. (S22) corresponds to

$$s_{i=\{x,y,z\}} = a_N - \sum_{\mathbf{k}} \frac{L(\mathbf{k})}{2\tilde{E}_{\mathbf{k}}^2}(\lambda_{i,\mathbf{k}}^2 - \sum_{j\neq i}\lambda_{j,\mathbf{k}}^2), \tag{S27}$$

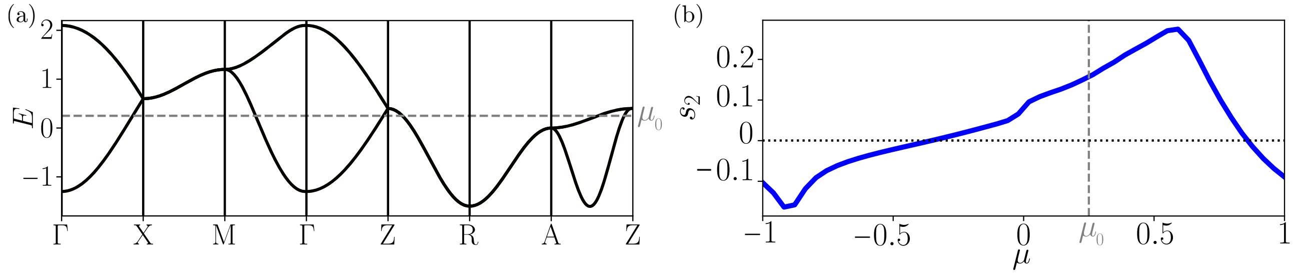


Figure S4. (a) Normal state band structure relevant for the rutile lattice (SG 136), using the tight-binding model in Table S2 and considering the hopping parameters in Table S3. (b) $s_2$ coefficient (see Eqs. (S23), (S28)) as a function of the chemical potential $\mu$ for the band structure shown in (a) and taking $T = 0.02$, $n_{\mathbf{k}} = 201^3$ and the SOC terms in Tables S2 - S3, displaying that the preferred direction for the Néel vector can switch by varying the Fermi energy.

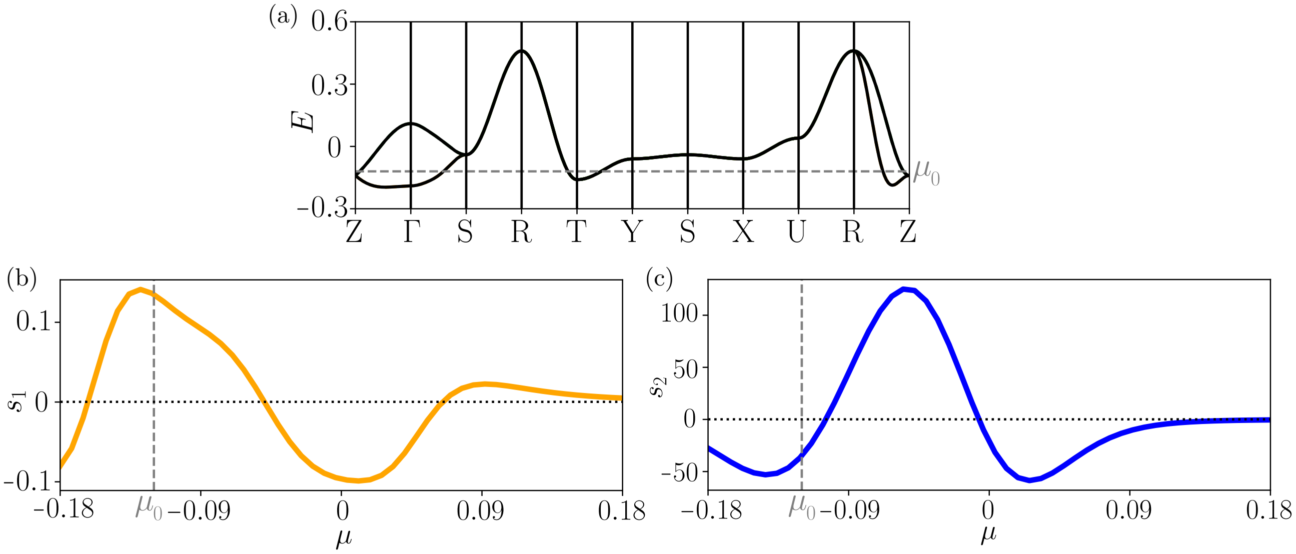


Figure S5. (a) Normal state band structure relevant for the $FeSb_2$ lattice (SG 58), using the tight-binding model in Table S2 and considering the hopping parameters in Table S3. (b)-(c) $s_1$ and $s_2$ coefficients (see Eqs. (S23), (S28)) as a function of $\mu$ for the band structure shown in (a) and taking $T = 0.02$, $n_{\mathbf{k}} = 201^3$ and the SOC terms in Tables S2 - S3, displaying that both the in-plane and out-of-plane preferred direction for the Néel vector can switch by varying the Fermi energy.

where the function $L(\mathbf{k})$ is defined in Eq. (8) of the main text. Thus, replacing this result in Eq. (S24),

$$\begin{aligned} s_0 &= a_N + \frac{1}{6}\sum_{\mathbf{k}} \frac{\lambda_{x,\mathbf{k}}^2 + \lambda_{y,\mathbf{k}}^2 + \lambda_{z,\mathbf{k}}^2}{\tilde{E}_{\mathbf{k}}^2} L(\mathbf{k}), \\ s_1 &= -\frac{1}{2}\sum_{\mathbf{k}} \frac{\lambda_{x,\mathbf{k}}^2 - \lambda_{y,\mathbf{k}}^2}{\tilde{E}_{\mathbf{k}}^2} L(\mathbf{k}), \\ s_2 &= -\frac{1}{6}\sum_{\mathbf{k}} \frac{\lambda_{x,\mathbf{k}}^2 + \lambda_{y,\mathbf{k}}^2 - 2\lambda_{z,\mathbf{k}}^2}{\tilde{E}_{\mathbf{k}}^2} L(\mathbf{k}). \end{aligned} \tag{S28}$$

In Fig. S4 and S5 we show the magnetic anisotropy coefficients for two different tight binding models. First, we focus on a model relevant for the rutile lattice (SG 136) with the band structure shown in Fig. S4(a). In this tetragonal case, the coefficient $s_1$ vanishes by symmetry, and $s_2$ determines the in-plane versus out-of-plane spin anisotropy. As seen from Fig. S4(b), for the chemical potential $\mu_0$ the preferred direction for the Néel vector is out-of-plane. However, for a lower $\mu$ it changes to in-plane, which may be due to the competition between the Linhard function and the density of states in the function $L(\mathbf{k})$. Considering now the tight-binding model inspired by the $FeSb_2$ band structure, see Fig. S5(a), for this orthorhombic material both coefficients $s_1$ and $s_2$ are generally non-zero. For the chemical

potential $\mu_0$, Figs. S5(b)-(c) show that the preferred direction of the altermagnetic moments is along the $y$ direction, but similar to the rutile case it can switch as a function of the Fermi energy.

---


[1] Matthias Hecker, Anant Rastogi, Daniel F. Agterberg, and Rafael M. Fernandes, "Classification of electronic nematicity in three-dimensional crystals and quasicrystals," Phys. Rev. B **109**, 235148 (2024).

[2] Ansgar Graf and Frédéric Piéchon, "Berry curvature and quantum metric in $N$-band systems: An eigenprojector approach," Phys. Rev. B **104**, 085114 (2021).

[3] Mercè Roig, Andreas Kreisel, Yue Yu, Brian M. Andersen, and Daniel F. Agterberg, "Minimal models for altermagnetism," Phys. Rev. B **110**, 144412 (2024).

[4] P. Blaha, K. Schwarz, G. K. Madsen, D. Kvasnicka, and J. Luitz, *WIEN2k an Augmented Plane Wave Plus Local Orbitals Program for Calculating Crystal Properties* (Technische Universität Wien, 2001).
